# Supplementary material for: Chemically Accurate Excitation Energies With Small Basis Sets
Source: arXiv:1907.01245 source file (2019-07-03)
Supplement: Supplementary file 1 [file Ex-srDFT-SI.pdf]

# Supporting Information for "Chemically Accurate Excitation Energies With Small Basis Sets"

Emmanuel Giner,[1, a)] Anthony Scemama,[2] Julien Toulouse,[1] and Pierre-François Loos[2, b)]
[1)] *Laboratoire de Chimie Théorique (UMR 7616), Sorbonne Université, CNRS, Paris, France*
[2)] *Laboratoire de Chimie et Physique Quantiques (UMR 5626), Université de Toulouse, CNRS, UPS, France*

## I. GEOMETRIES

Below are given the cartesian coordinates of the compounds investigated in this study. These are provided in Angstroms (Å) and they have been obtained at the CC3(full)/aug-cc-pVTZ level of theory,[1,2] except for methylene where the FCI/TZVP geometries have been extracted from Ref. 3.

### A. Ammonia

| | | | |
|---|---|---|---|
| N | 0.067759 | 0.000000 | 0.000000 |
| H | -0.313823 | 0.468746 | -0.811891 |
| H | -0.313823 | -0.937491 | 0.000000 |
| H | -0.313823 | 0.468746 | 0.811891 |

### B. Carbon dimer

| | | | |
|---|---|---|---|
| C | 0.000000 | 0.000000 | 0.624021 |
| C | 0.000000 | 0.000000 | -0.624021 |

### C. Ethylene

| | | | |
|---|---|---|---|
| C | 0.000000 | 0.666904 | 0.000000 |
| C | 0.000000 | -0.666904 | 0.000000 |
| H | 0.000000 | 1.229522 | 0.922291 |
| H | 0.000000 | -1.229522 | 0.922291 |
| H | 0.000000 | 1.229522 | -0.922291 |
| H | 0.000000 | -1.229522 | -0.922291 |

### D. Methylene

#### 1. $1\,^3B_1$ state

| | | | |
|---|---|---|---|
| C | 0.000000 | 0.000000 | 0.000000 |
| H | 0.000000 | 0.000000 | 1.077500 |
| H | -0.784304 | 0.000000 | -0.738832 |

#### 2. $1\,^1A_1$ state

| | | | |
|---|---|---|---|
| C | 0.000000 | 0.000000 | 0.000000 |
| H | 0.000000 | 0.000000 | 1.108900 |
| H | -1.085109 | 0.000000 | -0.228470 |

---

[a)]Corresponding author: emmanuel.giner@lct.jussieu.fr
[b)]Corresponding author: loos@irsamc.ups-tlse.fr

#### 3. $1\,^1B_1$ state

```
C     0.000000    0.000000    0.000000
H     0.000000    0.000000    1.074800
H    -0.668198    0.000000   -0.841847
```

#### 4. $2\,^1A_1$ state

```
C     0.000000    0.000000    0.000000
H     0.000000    0.000000    1.067800
H    -0.183953    0.000000   -1.051836
```

### E. Water

```
O    0.000000    0.000000   -0.069903
H    0.000000    0.757532    0.518435
H    0.000000   -0.757532    0.518435
```

## II. TOTAL ENERGIES

The exFCI total energies can be found in the supporting information of Refs. 1 and 2. Here, we report the absolute energetic corrections for each state of each molecule obtained with the three short-range correlation functionals considered in the present study (i.e., LDA, PBE-UEG and PBEot).

TABLE I. Total energies (in hartree) of excited states of methylene for various methods and basis sets. The value in parenthesis is an estimate on the last digit of the extrapolation error.

| | | States | | | |
|---|---|---|---|---|---|
| Method | Basis set | $1\,^3B_1$ | $1\,^1A_1$ | $1\,^1B_1$ | $2\,^1A_1$ |
| exFCI | AVDZ | −39.04846(1) | −39.03225(1) | −38.99203(1) | −38.95076(1) |
| | AVTZ | −39.08064(3) | −39.06565(2) | −39.02833(1) | −38.98709(1) |
| | AVQZ | −39.08854(1) | −39.07402(2) | −39.03711(1) | −38.99607(1) |
| | AV5Z | −39.09079(1) | −39.07647(1) | −39.03964(3) | −38.99867(1) |
| | CBS | −39.09141 | −39.07715 | −39.04034 | −38.99939 |
| exFCI+PBEot | AVDZ | −39.06924(1) | −39.05651(1) | −39.01777(1) | −38.97698(1) |
| | AVTZ | −39.08805(3) | −39.07430(2) | −39.03742(1) | −38.99652(1) |
| | AVQZ | −39.09189(1) | −39.07795(2) | −39.04124(1) | −39.00044(1) |
| exFCI+PBE-UEG | AVDZ | −39.07282(1) | −39.06150(1) | −39.02181(1) | −38.97873(1) |
| | AVTZ | −39.08948(3) | −39.07639(2) | −39.03911(1) | −38.99724(1) |
| | AVQZ | −39.09247(1) | −39.07885(2) | −39.04193(1) | −39.00066(1) |
| exFCI+LDA | AVDZ | −39.07450(1) | −39.06213(1) | −39.02233(1) | −38.97946(1) |
| | AVTZ | −39.09099(3) | −39.07779(2) | −39.04051(1) | −38.99859(1) |
| | AVQZ | −39.09319(1) | −39.07959(2) | −39.04267(1) | −39.00135(1) |

[1] Loos, P.-F.; Scemama, A.; Blondel, A.; Garniron, Y.; Caffarel, M.; Jacquemin, D. A Mountaineering Strategy to Excited States: Highly Accurate Reference Energies and Benchmarks. *J. Chem. Theory Comput.* **2018**, *14*, 4360–4379.
[2] Loos, P.-F.; Boggio-Pasqua, M.; Scemama, A.; Caffarel, M.; Jacquemin, D. Reference Energies for Double Excitations. *J. Chem. Theory Comput.* **2019**, *15*, 1939–1956.
[3] Sherrill, C. D.; Leininger, M. L.; Huis, T. J. V.; Schaefer, H. F. Structures and vibrational frequencies in the full configuration interaction limit: Predictions for four electronic states of methylene using a triple-zeta plus double polarization (TZ2P) basis. *J. Chem. Phys.* **1998**, *108*, 1040.

TABLE II. Basis set energetic corrections (in hartree) on vertical excitation energies for excited states of water, ammonia, carbon dimer, and ethylene for various methods and basis sets.

| | | Deviation with respect to TBE | | | | | | | | |
|---|---|---|---|---|---|---|---|---|---|---|
| | | exFCI+PBEot | | | exFCI+PBE-UEG | | | exFCI+LDA | | |
| Molecule | State | AVDZ | AVTZ | AVQZ | AVDZ | AVTZ | AVQZ | AVDZ | AVTZ | AVQZ |
| Water | $1\,^1A_1$ | −0.058 765 | −0.024 014 | −0.011 990 | −0.066 603 | −0.027 236 | −0.013 127 | −0.059 660 | −0.027 777 | −0.014 274 |
| | $1\,^1B_1$ | −0.052 137 | −0.021 369 | −0.010 611 | −0.061 033 | −0.025 180 | −0.012 076 | −0.054 803 | −0.025 596 | −0.013 154 |
| | $1\,^1A_2$ | −0.052 102 | −0.021 325 | −0.010 591 | −0.061 406 | −0.025 263 | −0.012 114 | −0.055 215 | −0.025 776 | −0.013 270 |
| | $2\,^1A_1$ | −0.052 995 | −0.021 690 | −0.010 852 | −0.061 959 | −0.025 457 | −0.012 258 | −0.055 301 | −0.025 786 | −0.013 304 |
| | $1\,^3B_1$ | −0.051 161 | −0.020 974 | −0.010 117 | −0.057 882 | −0.023 791 | −0.011 280 | −0.052 744 | −0.024 500 | −0.012 358 |
| | $1\,^3A_2$ | −0.051 244 | −0.020 982 | −0.010 115 | −0.058 090 | −0.023 847 | −0.011 302 | −0.052 729 | −0.024 611 | −0.012 398 |
| | $1\,^3A_1$ | −0.052 193 | −0.021 398 | −0.010 401 | −0.059 073 | −0.024 272 | −0.011 595 | −0.053 409 | −0.024 840 | −0.012 699 |
| Ammonia | $1\,^1A_1$ | −0.044 635 | −0.016 982 | −0.008 134 | −0.051 254 | −0.019 468 | −0.008 997 | −0.048 544 | −0.020 906 | −0.010 081 |
| | $1\,^1A_2$ | −0.039 461 | −0.014 997 | −0.007 039 | −0.047 284 | −0.018 061 | −0.008 251 | −0.044 515 | −0.019 266 | −0.009 218 |
| | $1\,^1E$ | −0.039 392 | −0.014 949 | −0.007 017 | −0.047 456 | −0.018 077 | −0.008 245 | −0.044 860 | −0.019 344 | −0.009 222 |
| | $2\,^1A_1$ | −0.040 071 | −0.014 995 | −0.006 988 | −0.047 916 | −0.018 163 | −0.008 241 | −0.045 561 | −0.019 651 | −0.009 258 |
| | $2\,^1A_2$ | −0.039 483 | −0.014 904 | −0.006 961 | −0.047 307 | −0.018 019 | −0.008 211 | −0.045 008 | −0.019 252 | −0.009 175 |
| | $1\,^3A_2$ | −0.038 969 | −0.014 725 | −0.006 828 | −0.047 144 | −0.018 010 | −0.008 221 | −0.044 361 | −0.019 216 | −0.009 181 |
| Carbon dimer | $1\,^1\Sigma_g^+$ | −0.037 716 | −0.014 339 | −0.006 758 | −0.050 128 | −0.019 217 | −0.008 918 | −0.049 570 | −0.021 425 | −0.010 307 |
| | $1\,^1\Delta_g$ | −0.042 611 | −0.016 313 | −0.007 592 | −0.050 686 | −0.019 737 | −0.009 079 | −0.049 710 | −0.021 590 | −0.010 380 |
| | $2\,^1\Sigma_g^+$ | −0.042 167 | −0.016 136 | −0.00 7567 | −0.050 333 | −0.019 473 | −0.00 8978 | −0.049 208 | −0.021 292 | −0.01 0257 |
| Ethylene | $1\,^1A_{1g}$ | −0.057 559 | −0.022 007 | | −0.066 251 | −0.024 599 | | −0.065 343 | −0.027 274 | |
| | $1\,^1B_{3u}$ | −0.054 862 | −0.020 972 | | −0.063 185 | −0.023 501 | | −0.061 786 | −0.025 978 | |
| | $1\,^1B_{1u}$ | −0.057 591 | −0.022 249 | | −0.064 517 | −0.023 971 | | −0.063 619 | −0.026 561 | |
| | $1\,^1B_{1g}$ | −0.054 995 | −0.020 994 | | −0.063 386 | −0.023 564 | | −0.061 978 | −0.026 087 | |
| | $1\,^3B_{1u}$ | −0.056 056 | −0.020 862 | | −0.063 499 | −0.023 241 | | −0.063 304 | −0.025 971 | |
| | $1\,^3B_{3u}$ | −0.054 752 | −0.020 441 | | −0.062 078 | −0.022 891 | | −0.060 894 | −0.025 249 | |
| | $1\,^3B_{1g}$ | −0.054 924 | −0.020 480 | | −0.062 306 | −0.022 962 | | −0.061 089 | −0.025 334 | |
